# Supplementary material for: EDA: Easy Data Augmentation Techniques for Boosting Performance on Text Classification Tasks
Source: arXiv:1901.11196 source file (2019-08-25)
Supplement: Supplementary file 1 [file rnn_supp.tex]

\begin{table}[ht]
\centering
\begin{tabular}{l|c}
\hline
Epochs & Early stopping \\ \hline
Loss & Categorical cross-entropy \\ \hline
Optimizer & Adam \\ \hline
Activation & ReLU \\ \hline
Initialization & Random normal \\ \hline
\end{tabular}
\caption{RNN model hyperparameters.}
\label{tab:rnn_supp}
\end{table}
